# Supplementary material for: Understanding and Resolving Performance Degradation in Graph Convolutional Networks
Source: arXiv:2006.07107 source file (2021-09-13)
Supplement: Supplementary file 1 [file supp.tex]

\clearpage

\section{Layernorm}

We can also see from Fig.~\ref{fig:address-performance-degradation} that LayerNorm achieves comparable results with \nodenormone in most of the experiments. 
However, since LayerNorm performs three operations, more investigation is needed to demonstrate reducing \varianceinflaming is the key to the effectiveness of LayerNorm in resolving performance degradation of deep GCNs. 
We then ablatively study the effects of the three kinds of operations in LayerNorm on addressing performance degradation.
Specifically, we study two variants of LayerNorm: 
\begin{equation}
    % \vspace{-5mm}
    \begin{aligned}
    \mathrm{LayerNorm}^*({\mathbf{h}_i}) = \frac{\mathbf{h}_i - \mu_i}{\sigma_i},
    \end{aligned}
    \label{eqn:layernorm*}
\end{equation}
\begin{equation}
    % \vspace{-5mm}
    \begin{aligned}
    \mathrm{LayerNorm\text{-}MS}({\mathbf{h}_i}) = \mathbf{h}_i - \mu_i.
    \end{aligned}
    \label{eqn:layernorm-ms}
\end{equation}

\begin{figure}
    \centering
    \includegraphics[width=\linewidth]{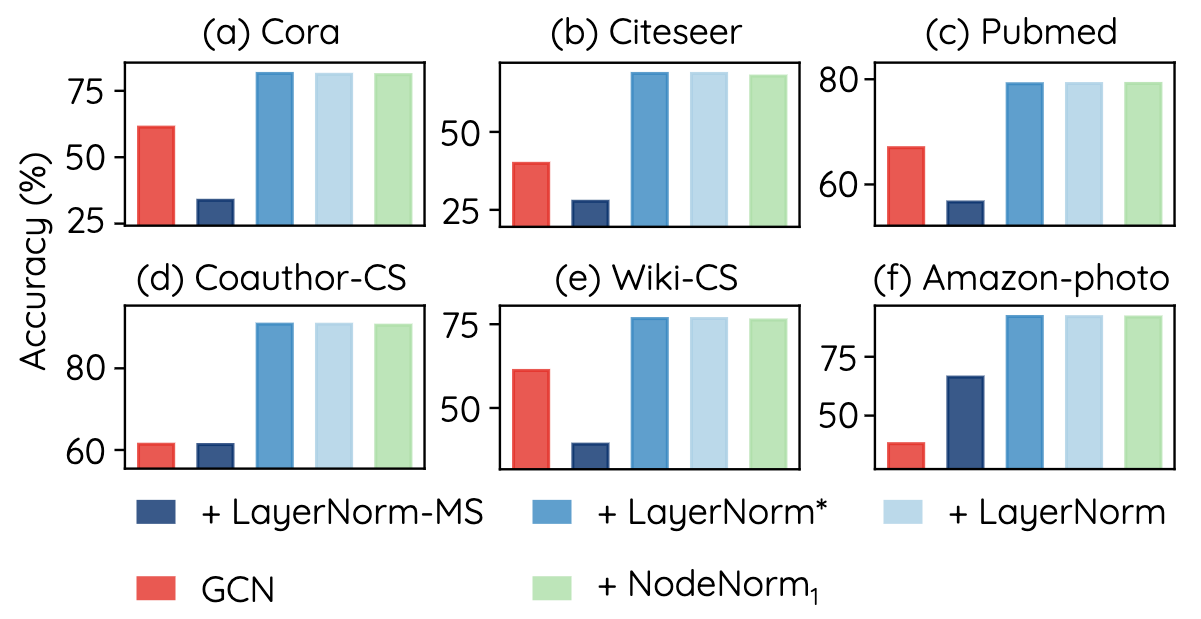}
    \caption{Classification accuracy of 64-layer GCNs with LayerNorm-MS and LayerNorm*. We also include results of the baseline GCNs, GCNs with \nodenormone or LayerNorm for clearer comparison.}
    \label{fig:layernorm-ms}
\end{figure}
The LayerNorm* variant does not include linear transformations, while the LayerNorm-MS variant performs only Mean-Subtraction (MS).

We conduct experiments with the two variants of 64 layers, with the same settings as in Sec.~\ref{subsubsec:address-pd-exp-settings}, and show results in Fig.~\ref{fig:layernorm-ms}.
We can see that GCNs with LayerNorm*, LayerNorm or \nodenormone perform comparatively, while those with LayerNorm-MS perform significantly worse (on 4 datasets even worse than baseline GCNs).
Note that \nodenormone is equivalent to the variance-scaling step in LayerNorm.
Moreover, we also find that the linear transformation is trained to approximate identity mappings, which will be elaborated in Supplementary Materials. 
The above observations show that linear transformation and the mean-subtraction step are not critical for improving deep GCNs performance; instead, variance-scaling is the step that really works. 
This further demonstrates that reducing \varianceinflaming is the key to addressing performance degradation.

\section{More insights on mitigating variance inflammation}
\label{sec:analysis}
\subsection{Where to put variance-controlling techniques}
\label{subsec:where-to-control-the-variance}
Normalization operations~\cite{ioffe2015batch, ba2016layer} are generally put after convolution layers in the literature of GNNs.
Following this convention, in experiments in Sec.~\ref{sec:experiments}, we put variance-controlling techniques, \ie, \nodenorm and LayerNorm, after each Graph Convolutional~(GC) layer (after the \tran of each layer), and show that this effectively addresses \varianceinflaming and performance degradation. 

\begin{figure*}[t!]
\centering
    \includegraphics[width=\linewidth]{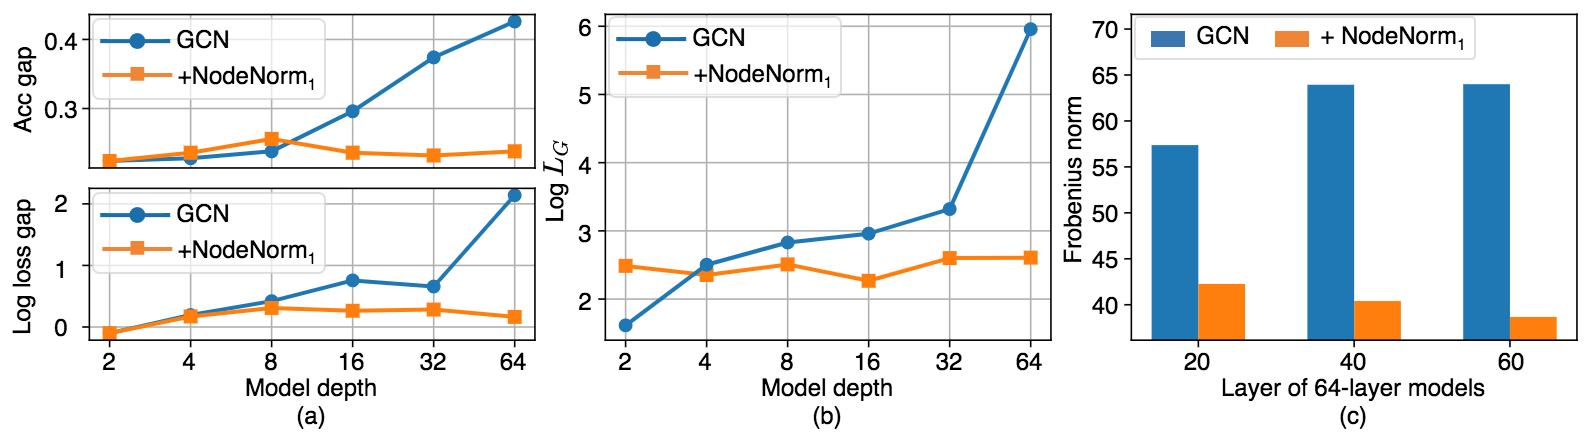}
    \caption{(a)~Accuracy gap (upper) and loss gap (lower) of GCNs between training and validation set. Note,
loss gap is shown in a log scale with base of 10. 
(b)~Graph Lipschitz constant ($L_G$) of models with different depths. 
Results are in log scale with base of 10.
(c)~Frobenius norm of feature correlation matrices of different hidden layers of 64-layer models.
Results are on Cora.
See Supplementary Materials for results on Citeseer and Pubmed.}
\label{fig:reduce-overfitting}
\end{figure*}
\begin{table}[t!]
    \caption{Classification accuracy of 64-layer GCNs with \nodenormonein, \nodenormone LayerNorm-In, or LayerNorm on Cora, Citeseer and Pubmed. We also include results of \nodenormone and LayerNorm for clearer comparison, which are from Tab.~\ref{fig:address-performance-degradation}.}
    \label{tab:inside-conv-norm}
    \centering
    \resizebox{0.90\linewidth}{!}{
    \begin{small}
    \begin{tabular}{|c|c|c|c|}
    \hline
           & Cora & Citeseer & Pubmed \\
          \hline
          \nodenormonein & 0.8104 & 0.6901 & 0.7913\\
          \hline
          \nodenormone & 0.8108 & 0.6790 & 0.7920\\
          \hline
          \hline
          LayerNorm-In & 0.8036 & 0.6901 & 0.7945\\
          \hline
          LayerNorm & 0.8122 & 0.6875 & 0.7918\\
          \hline
    \end{tabular}
    \end{small}
    }
\end{table}

We note that placing variance-controlling techniques before the \tran of each GC layer can also prevent node-wise variance from being amplified layer by layer, which also mitigates \varianceinflaming.
This yields a GC layer with a variance-controlling technique placed \textit{inside} it:
\begin{equation}
    \begin{aligned}
    H^{(l)} = \mathrm{ReLU}(f(\hat{A}H^{(l-1)})W^{(l)}),
    \end{aligned}
    \label{eqn:GC-layer-with-nodenorm}
\end{equation} 
where $f(\cdot)$ can be a \nodenorm or LayerNorm operation.
We refer to this implementation of \nodenormp and LayerNorm as \nodenormpin and LayerNorm-In respectively (``In'' for ``Inside GC'').

To justify that this implementation also helps alleviate performance degradation, we conduct experiments of GCNs of layers \{2, 4, 8, 16, 32, 64\} equipped with \nodenormpin and LayerNorm-In on Cora, Citeseer and Pubmed with the 20-label-per-class setting introduced in Sec.~\ref{subsubsec:address-pd-exp-settings}.
We take \nodenormone as an example of \nodenormp because it outperforms \nodenormp with other values of $p$ (see Sec.\ref{subsec:address-performance-degradation}).

As shown in Tab.~\ref{tab:inside-conv-norm}, \nodenormonein and LayerNorm-In achieve comparable results with \nodenormone and LayerNorm respectively. 
This shows this inside convolution implementation of variance-controlling techniques also effectively resolves performance degradation.

We believe the above results provide valuable insights to the community of GNNs: normalization operations do not necessarily need to be placed after convolution layers as in CNNs.

\subsection{Other benefits of mitigating variance inflammation}
\label{subsec:reduce-overfitting}

As pointed out in~\cite{klicpera2018predict, zhao2019pairnorm}, deep GCNs tend to suffer more overfitting than shallow ones, which is also a factor contributing to performance degradation. 
Existing works generally tackle overfitting by regularization techniques such as Dropout~\cite{srivastava2014dropout}. 
We find that mitigating \varianceinflaming also helps reduce overfitting. 
We take \nodenormone as an example to illustrate this.

We first show overfitting in GCNs via loss gap and accuracy gap between train split and validation split. 
We run experiments on Cora, Citeseer and Pubmed, and show the results in Fig.~\ref{fig:reduce-overfitting}.
Comparing the curves in Fig.~\ref{fig:reduce-overfitting}~(a), we can see \nodenormone effectively mitigates overfitting in deep GCNs.

We then experimentally investigate how \nodenormone achieves this from two perspectives: characteristics of models, and characteristics of hidden features.
From the perspective of model characteristics, we define the Graph Lipschitz Constant, denoted as $L_G$, for GNNs to measure their smoothness w.r.t. node features, which is inspired by observations in~\cite{bartlett2017spectrally, gouk2018regularisation, zou2019lipschitz} that the networks enforced to have lower Lipschitz constant\footnote{A function $f(\mathbf{x})$ is $L$-Lipschitz if $\|f(\mathbf{x}_1) - f(\mathbf{x}_2)\| \leqslant L\|\mathbf{x}_1 - \mathbf{x}_2\|,\forall \mathbf{x}_1, \mathbf{x}_2$. $L$ is the Lipschitz constant.} tend to have better generalization ability and suffer less overfitting.
We investigate how \nodenormone affects model smoothness.

Let $f(\mathbf{x}, G; \mathbf{w})$ denote a GNN, where $\mathbf{x}$ is the input node feature vector, $G$ is the input graph structure and $\mathbf{w}$ is the model parameters. 
For a given graph $G$, the $L_G$ is 
\begin{equation}
\label{eqn:lg}
    \begin{aligned}
    L_G = \max_{i,j \in V}\frac{\|f(\mathbf{x}_i;G,\mathbf{w}) - f(\mathbf{x}_j;G,\mathbf{w})\|}{\|\mathbf{x}_j - \mathbf{x}_j\|}.
    \end{aligned}
\end{equation}
From Eqn.~\eqref{eqn:lg}, the models with smaller $L_G$ are less sensitive to disturbances in node features. 
We compare the $L_G$ values of GCNs with or without \nodenormone, as shown in Fig.~\ref{fig:reduce-overfitting}~(b). 
We can see \nodenormone effectively reduces $L_G$ and acts as an implicit regularizer in the training process of deep models.

From the perspective of characteristics of hidden features, inspired by observing that overfitting can be alleviated by decorrelating hidden features~\cite{cogswell2015reducing}, we investigate whether \nodenormone can reduce feature correlation. 
We compare the correlation among hidden features of 64-layer GCNs with or without \nodenormone.
Specifically, we compute the Frobenius norm of feature correlation matrices of different layers of the two models, as shown in Fig.~\ref{fig:reduce-overfitting}~(c). 
It can be seen the model trained with \nodenormone has less correlated features than others, showing \nodenormone can effectively reduce overfitting.

\begin{table}[t!]
    \centering
    \caption{Statistics of datasets used in this section. 
    The task is multi-class classification on all the datasets except Ogbn-proteins dataset (marked with $^\dagger$) where multi-label classification is performed, \ie,  112 independent binary classification tasks.}
    \label{tab:dataset statistics}
    \resizebox{1.0\linewidth}{!}{
    \begin{tabular}{|c|c|c|c|c|c|}
    \hline
         Datasets & \#Nodes &\#Edges & \makecell{\#Node \\ features} & \makecell{\#Edge \\ features} & \#Classes \\
     \hline
     Cora & 2,708 & 5,278 & 1,433 & - & 7 \\
     \hline
     Citeseer & 3,327 & 4,551 & 3,703 & - & 6 \\
     \hline
     Pubmed & 19,717 & 44,324 & 500 & - & 3 \\
     \hline
     Coauthor-CS & 18,333 & 81,894 & 6,805& - & 15 \\
     \hline
     Amazon-photo & 7650 & 119,081 & 767 & - & 10 \\
     \hline
     Wiki-CS &  11,701 & 216,123 & 300 & - & 10 \\
     \hline
     US-election12 & 3,234 & 12,717 & 6 & - & 2 \\
     \hline 
     US-election16 & 3,234 & 12,717 & 6 & - & 2 \\
     \hline 
     Ogbn-proteins & 132,534 & 39,561,252 & - & 8 & 112$^\dagger$ \\
     \hline
     Cornell & 183 & 295 & 1,703 & - & 5 \\
     \hline
     Texas & 183 & 309 & 1,703 & - & 5 \\
     \hline
     Wisconsin & 251 & 499 & 1,703 & - & 5 \\
     \hline 
    \end{tabular}
    }
\end{table}

\section*{Supplementary Materials}
In Supplementary Materials~A~(SM.~A), we show results of analytical experiments in Sec.~3 on other datasets. Then in SM.~B we give  numerical results of figures in Sec.4, and some supplementary experimental results. Next, we implementation details of our experiments in Sec.~4 in SM.~C. 

\subsection*{A Analytical experiments on other datasets}
In Sec.3, we use Cora dataset to illustrate our observations. Here we show corresponding results on Citeseer, Pubmed, Coauthor-CS, Wiki-CS and Amazon-photo.
\subsubsection*{A.1 TRANs contribute significantly to performance degradation}
Fig. 7 shows performance degradation of GCNs, P-GCNs and T-GCNs on the aforementioned datasets.
\subsubsection*{A.2 TRANs tend to amplify node-wise variance}
Fig. 8 shows that TRANs tend to amplify node-wise variance $\mathrm{var}_i$.
\subsubsection*{A.3 Variance inflaming}
Fig.9 shows \varianceinflaming of GCNs on these datasets.

\subsection*{B Supplementary results for Sec.~4}
\subsubsection*{B.1 Numerical results}
Tab.~9 shows numerical results (including standard deviation) for Fig~3. Tab.~10 to Tab.~14 show standard deviation for results in Tab.~2, Tab.~3, Tab.~4, Tab.~6 and Tab.~7 respectively.

\subsubsection*{B.2 Further Comparisons with best competing methods}
We conduct further comparisons with current best competing methods (i.e. PairNorm and Dropedge) in cases where deeper models are desired. To be more specific, we compare our method with them in two scenarios. The first one is a low training label rate setting when only 2 labels per class are available, and the second one is when all non-training features are missing. As Tab.~\ref{tab:further-sota} shows, models augmented with \nodenormone are superior to all other methods in most of the scenarios.

\subsubsection*{B.3 Visualizing learned parameters in LayerNorm}
As mentioned in Sec.~4.1.2, the feature-wise linear transformation in LayerNorm are trained to approximate identity mappings. Here we elaborate this observation by visualizing the learned parameters in LayerNorm. Specifically, we visualize entries of $\mathbf{\alpha}$ and $\mathbf{\beta}$ of the LayerNorm in the different hidden layers layer of a 64-layer trained GCN model in Fig.~10. We can see that entries of $\alpha$ are close 1, while thoes of $\beta$ are close to. Consequently, the feature-wise linear transformation approximates an identical mapping.

\subsubsection*{B.4 Scenarios where larger $p$ in \nodenormp is desired}
From experimental results in Sec.~4, we can see that \nodenormone brings more performance improvement of deep GCNs (\eg 64-layer) than \nodenormtwo and \nodenormthree. This is because deep GCNs suffer suffer severe \varianceinflaming, and thus techniques that controlling variance more strictly brings more performance gain. However, in scenarios where \varianceinflaming is less severe, \nodenormp with larger $p$ which is less strict than \nodenormone, would be more desired. This is evidenced by Tab.~9: for shallow models (\eg 2-layer, 4-layer, 8-layer), GCNs with \nodenormthree and \nodenormtwo generally achieves better than those with \nodenormone. This demonstrates that \nodenorm is flexible. Indeed, we can control the value of $p$ so that \nodenormp collaborate well with GCNs in different scenarios.

\subsubsection*{B.5 Supplementary results for Sec.~5.2}
In Fig.~11 and Fig.~12, we show results of analytical experiments in Sec.~5.2 on Citeseer and Pubmed respectively.

\subsection*{Implementation details}
In Tab.~15 to Tab.~22, we list hyperparameters used in Sec.~4. The hyperparameters are obtained by grid search. 

% \begin{strip}
% \centering
% \includegraphics[width=1.0\linewidth]{Figures/supp/supp_trans_more.png}
% \captionof{figure}{Classification accuracy \wrt model depth.}
% \end{strip}

\onecolumn
\begin{figure}[h!]
\centering
    \includegraphics[width=0.9\linewidth]{Figures/supp/supp_trans_more.png}
    \caption{Classification accuracy \wrt model depth.}
\end{figure}
\begin{figure}[h!]
\centering
    \includegraphics[width=0.9\linewidth]{Figures/supp/supp_trans_amplify.png}
    \caption{Node-wise variance, \ie, $\mathrm{var}_i^{(l)}$ of all nodes in different layers ($l=1, 20, 40, 60$) of 64-layer T-GCN and P-GCN models. Results are shown in log scale with a base of 10.}
\end{figure}
\begin{figure}[h!]
\centering
    \includegraphics[width=0.9\linewidth]{Figures/supp/supp_variance_inflaming.png}
    \caption{Node-wise variance of the last layer, \ie, $\mathrm{var}_i^{(L)}$ (in log scale with a base of 10) for $L=2, 4, 8, 16, 32, 64$ of all nodes.}
\end{figure}

\clearpage
\onecolumn
\subsection*{B Supplementary experimental results}
% In this subsection, we give supplementary experimental results, including numerical results of figures, and standard deviations of tables in Sec.~4.
\subsubsection*{B.1 Numerical results}
% fig.3 results
\begin{table}[h]
  \caption{Numerical results of Fig.~3.}
%   \label{tab:ablation}
  \centering
  \resizebox{0.85\linewidth}{!}{%
  \begin{tabular}{|l|l|c|c|c|c|c|c|}
    \hline                  
    %\cmidrule(r){1-2}
    	     
		 Method & Dataset & 2-Layer & 4-Layer & 8-Layer & 16-Layer & 32-Layer & 64-Layer \\
		%& & \multicolumn{4}{c}{\bf CIFAR-10} & \multicolumn{4}{c}{\bf CIFAR-100} \\ 
		\hline
		        \multirow{6}{*}{GCN} 
				& Cora & 81.09{\scriptsize $\pm$0.85} & 80.74{\scriptsize $\pm$1.87} & 80.03{\scriptsize $\pm$1.56} & 74.72{\scriptsize $\pm$2.63} & 63.74{\scriptsize $\pm$1.79} & 61.13{\scriptsize $\pm$3.28} \\
				& Citeseer & 70.97{\scriptsize $\pm$1.16} & 67.70{\scriptsize $\pm$1.49} & 66.45{\scriptsize $\pm$1.50} & 61.75{\scriptsize $\pm$2.71} & 41.83{\scriptsize $\pm$4.53} & 39.92{\scriptsize $\pm$2.06} \\
				& Pubmed & 77.76{\scriptsize $\pm$2.36} & 77.44{\scriptsize $\pm$2.22} & 78.09{\scriptsize $\pm$1.53} & 73.55{\scriptsize $\pm$4.38} & 70.22{\scriptsize $\pm$2.95} & 66.99{\scriptsize $\pm$4.24} \\
				& Coauthor-CS & 91.30{\scriptsize $\pm$0.65} & 90.04{\scriptsize $\pm$0.58} & 88.69{\scriptsize $\pm$0.91} & 84.44{\scriptsize $\pm$1.36} & 70.54{\scriptsize $\pm$5.05} & 61.41{\scriptsize $\pm$3.15} \\
				& Wiki-CS & 76.98{\scriptsize $\pm$0.65} & 76.20{\scriptsize $\pm$0.54} & 75.99{\scriptsize $\pm$0.63} & 76.09{\scriptsize $\pm$0.72} & 76.13{\scriptsize $\pm$0.69} & 76.25{\scriptsize $\pm$0.64}  \\
				& Amazon-photo & 91.46{\scriptsize $\pm$1.07} & 90.82{\scriptsize $\pm$0.93} & 88.62{\scriptsize $\pm$1.36} & 85.86{\scriptsize $\pm$2.17} & 83.59{\scriptsize $\pm$2.11} & 38.08{\scriptsize $\pm$10.64} \\
				\hline
				\multirow{6}{*}{+\nodenormone} 
				& Cora & 80.48{\scriptsize $\pm$1.23} & 80.58{\scriptsize $\pm$1.71} & 80.96{\scriptsize $\pm$1.62} & 80.16{\scriptsize $\pm$1.04} & 80.13{\scriptsize $\pm$0.84} & 81.08{\scriptsize $\pm$1.87} \\
				& Citeseer & 69.34{\scriptsize $\pm$1.02} & 68.34{\scriptsize $\pm$2.80} & 68.85{\scriptsize $\pm$1.82} & 68.50{\scriptsize $\pm$1.83} & 69.28{\scriptsize $\pm$1.63} & 67.90{\scriptsize $\pm$1.84}  \\
				& Pubmed & 79.97{\scriptsize $\pm$1.44} & 78.61{\scriptsize $\pm$2.19} & 79.98{\scriptsize $\pm$0.94} & 78.35{\scriptsize $\pm$1.68} & 78.55{\scriptsize $\pm$2.14} & 79.20{\scriptsize $\pm$2.37}  \\
				& Coauthor-CS & 92.12{\scriptsize $\pm$0.35} & 91.06{\scriptsize $\pm$0.92} & 91.36{\scriptsize $\pm$0.37} & 91.22{\scriptsize $\pm$0.46} & 91.17{\scriptsize $\pm$0.52} & 90.59{\scriptsize $\pm$0.81}  \\
				& Wiki-CS& 77.43{\scriptsize $\pm$0.68} & 76.56{\scriptsize $\pm$0.63} & 75.99{\scriptsize $\pm$0.62} & 75.05{\scriptsize $\pm$0.71} & 72.53{\scriptsize $\pm$2.38} & 68.26{\scriptsize $\pm$3.15} \\
				& Amazon-photo & 92.05{\scriptsize $\pm$1.14} & 92.07{\scriptsize $\pm$0.62} & 91.10{\scriptsize $\pm$0.84} & 91.68{\scriptsize $\pm$0.71} & 91.76{\scriptsize $\pm$0.91} & 91.88{\scriptsize $\pm$1.31} \\
				\hline
				\multirow{6}{*}{+\nodenormtwo} 
				& Cora & 81.17{\scriptsize $\pm$1.77} & 80.96{\scriptsize $\pm$1.86} & 81.25{\scriptsize $\pm$1.90} & 80.41{\scriptsize $\pm$0.92} & 80.01{\scriptsize $\pm$1.44} & 79.69{\scriptsize $\pm$2.59} \\
				& Citeseer & 69.91{\scriptsize $\pm$2.09} & 68.66{\scriptsize $\pm$1.99} & 68.34{\scriptsize $\pm$1.97} & 68.19{\scriptsize $\pm$2.04} & 68.48{\scriptsize $\pm$1.96} & 65.92{\scriptsize $\pm$0.66} \\
				& Pubmed & 80.61{\scriptsize $\pm$1.50} & 78.65{\scriptsize $\pm$1.27} & 79.67{\scriptsize $\pm$1.51} & 77.74{\scriptsize $\pm$2.55} & 77.74{\scriptsize $\pm$1.94} & 77.83{\scriptsize $\pm$2.57}  \\
				& Coauthor-CS& 92.43{\scriptsize $\pm$0.32} & 90.40{\scriptsize $\pm$0.99} & 90.10{\scriptsize $\pm$0.31} & 89.56{\scriptsize $\pm$0.60} & 89.22{\scriptsize $\pm$0.71} & 88.41{\scriptsize $\pm$0.45} \\
				& Wiki-CS & 77.40{\scriptsize $\pm$0.71} & 76.78{\scriptsize $\pm$0.52} & 75.74{\scriptsize $\pm$0.47} & 71.41{\scriptsize $\pm$2.82} & 70.66{\scriptsize $\pm$2.38} & 67.76{\scriptsize $\pm$1.91}  \\
				& Amazon-photo & 92.17{\scriptsize $\pm$0.85} & 91.95{\scriptsize $\pm$0.64} & 90.59{\scriptsize $\pm$1.60} & 91.00{\scriptsize $\pm$0.96} & 90.31{\scriptsize $\pm$1.05} & 89.91{\scriptsize $\pm$1.86}  \\
				\hline
				\multirow{6}{*}{+\nodenormthree} 
				& Cora & 81.13{\scriptsize $\pm$1.12} & 81.47{\scriptsize $\pm$1.37} & 81.43{\scriptsize $\pm$1.59} & 79.45{\scriptsize $\pm$1.80} & 73.84{\scriptsize $\pm$3.48} & 73.55{\scriptsize $\pm$4.09} \\
				& Citeseer & 69.86{\scriptsize $\pm$0.83} & 68.98{\scriptsize $\pm$1.49} & 67.80{\scriptsize $\pm$1.81} & 66.52{\scriptsize $\pm$2.31} & 59.45{\scriptsize $\pm$10.36} & 62.64{\scriptsize $\pm$3.36} \\
				& Pubmed & 80.33{\scriptsize $\pm$1.76} & 78.46{\scriptsize $\pm$1.86} & 79.59{\scriptsize $\pm$1.48} & 77.63{\scriptsize $\pm$2.23} & 76.34{\scriptsize $\pm$2.31} & 75.54{\scriptsize $\pm$3.71} \\
				& Coauthor-CS & 92.36{\scriptsize $\pm$0.40} & 90.51{\scriptsize $\pm$0.63} & 89.06{\scriptsize $\pm$0.74} & 88.82{\scriptsize $\pm$0.56} & 87.64{\scriptsize $\pm$0.61} & 85.59{\scriptsize $\pm$1.27}  \\
				& Wiki-CS & 77.14{\scriptsize $\pm$0.62} & 76.76{\scriptsize $\pm$0.41} & 76.68{\scriptsize $\pm$0.67} & 76.59{\scriptsize $\pm$0.62} & 76.95{\scriptsize $\pm$0.50} & 76.70{\scriptsize $\pm$0.56}  \\
				& Amazon-photo & 92.15{\scriptsize $\pm$0.94} & 91.81{\scriptsize $\pm$0.95} & 90.21{\scriptsize $\pm$1.19} & 90.02{\scriptsize $\pm$1.65} & 87.45{\scriptsize $\pm$2.22} & 83.91{\scriptsize $\pm$2.69}\\
				\hline
				\multirow{6}{*}{+LayerNorm} 
				& Cora & 80.46{\scriptsize $\pm$1.10} & 80.80{\scriptsize $\pm$1.47} & 80.63{\scriptsize $\pm$0.95} & 80.36{\scriptsize $\pm$1.54} & 79.91{\scriptsize $\pm$1.38} & 81.22{\scriptsize $\pm$1.54}  \\
				& Citeseer & 69.49{\scriptsize $\pm$1.14} & 68.65{\scriptsize $\pm$1.79} & 69.25{\scriptsize $\pm$2.02} & 68.94{\scriptsize $\pm$1.62} & 69.82{\scriptsize $\pm$1.77} & 68.75{\scriptsize $\pm$1.25} \\
				& Pubmed & 80.07{\scriptsize $\pm$1.49} & 79.10{\scriptsize $\pm$2.03} & 79.73{\scriptsize $\pm$1.19} & 78.69{\scriptsize $\pm$1.72} & 78.86{\scriptsize $\pm$1.05} & 79.18{\scriptsize $\pm$2.02}\\
				& Coauthor-CS& 92.19{\scriptsize $\pm$0.65} & 91.12{\scriptsize $\pm$0.84} & 91.40{\scriptsize $\pm$0.43} & 91.14{\scriptsize $\pm$0.45} & 91.29{\scriptsize $\pm$0.47} & 90.80{\scriptsize $\pm$0.66}  \\
				& Wiki-CS & 77.14{\scriptsize $\pm$0.62} & 76.76{\scriptsize $\pm$0.41} & 76.68{\scriptsize $\pm$0.67} & 76.59{\scriptsize $\pm$0.62} & 76.95{\scriptsize $\pm$0.50} & 76.70{\scriptsize $\pm$0.56}  \\
				& Amazon-photo & 92.14{\scriptsize $\pm$1.04} & 92.25{\scriptsize $\pm$0.62} & 91.30{\scriptsize $\pm$0.97} & 91.71{\scriptsize $\pm$1.28} & 91.93{\scriptsize $\pm$0.70} & 92.05{\scriptsize $\pm$1.05}  \\
    \hline
  \end{tabular}}
\end{table}
\begin{table}[h]
    \centering
    \caption{Further comparisons with best competing methods. We conduct experiments on two scenarios where deeper models are desired: 1) when only 2 training labels per class are available, 2) when feature missing rate is 100\%.}
    \label{tab:further-sota}
    \begin{tabular}{|c|c|c|c|c|c|}
    \hline
         \multirow{2}{*}{Dataset}& \multirow{2}{*}{Scenario} &\multicolumn{4}{c|}{Method}\\
    \cline{3-6}
    && GCN  & +PairNorm &+DropEdge & +\nodenormone\\
    \hline
    \multirow{2}{*}{Cora} & Low label rate  & 0.6319 (4)  &0.5777 (16)&0.6193 (4)& \textbf{0.6420 (16)}\\
    \cline{2-6}
     & Missing features & 0.7034 (8)  &0.6847 (64)&\textbf{0.7335 (16)}& 0.7207 (64)\\
    \hline
    \multirow{2}{*}{Citeseer}& Low label rate & 0.5277 (2)  &0.4805 (8)&0.4710 (8)& \textbf{0.5516 (16)}\\
    \cline{2-6}
     & Missing features & 0.4429 (8)  &0.4475 (32)&0.4811 (16)& \textbf{0.4861 (32)}\\
    \hline
    \multirow{2}{*}{Pubmed}  & Low label rate & 0.6491 (4)  &0.6525 (32)&0.6557 (4)& \textbf{0.6813 (64)}\\     \cline{2-6}
     & Missing features & 0.4652 (16) & \textbf{0.6683 (32)}&0.4292 (32)& 0.5751 (16) \\
    \hline
    \end{tabular}
\end{table}

% \begin{table}[h]
%     \centering
%     \caption{Further comparisons with best competing methods. We conduct experiments on two scenarios where deeper models are desired: 1) when only 2 training labels per class are available, 2) when feature missing rate is 100\%.}
%     \label{tab:further-sota}
%     \begin{tabular}{|c|c|c|c|c|c|c|c|}
%     \hline
%          \multirow{2}{*}{Dataset}& \multirow{2}{*}{Scenario} &\multicolumn{4}{c|}{Method}\\
%     \cline{3-8}
%     && GCN  & +PairNorm &+DropEdge & +\nodenormone &+\nodenormtwo &+\nodenormthree\\
%     \hline
%     \multirow{2}{*}{Cora} & Low label rate  & 0.6319 (4)  &0.5777 (16)&0.6193 (4)& 0.6420 (16) &\textbf{0.6605 (16)}& 0.6580 (8)\\
%     \cline{2-8}
%      & Missing features & 0.7034 (8)  &0.6847 (64)&0.7335 (16)& 0.7207 (64) &\textbf{ 0.7361 (16)}\\
%     \hline
%     \multirow{2}{*}{Citeseer}& Low label rate & 0.5277 (2)  &0.4805 (8)&0.4710 (8)& 0.5516 (16) &0.5551 (4)& \textbf{0.5616 (4)}\\
%     \cline{2-8}
%      & Missing features & 0.4429 (8)  &0.4475 (32)&0.4811 (16)& 0.4861 (32) & 0.4987 (32)\\
%     \hline
%     \multirow{2}{*}{Pubmed}  & Low label rate & 0.6491 (4)  &0.6525 (32)&0.6557 (4)& 0.6813 (64) &\textbf{0.6908 (32)}& 0.6694 (8)\\     \cline{2-8}
%      & Missing features & 0.4652 (16) & \textbf{0.6683 (32)}&0.4292 (32)& 0.5751 (16) & 0.6106 (16)\\
%     \hline
%     \end{tabular}
% \end{table}

\clearpage
\twocolumn

\begin{table}[h]
    \centering
    \caption{Standard deviation of results in Tab.~2.}
    \label{tab:missing-features-supp}
    \begin{tabular}{|c|c|c|c|}
    \hline
         \multirow{2}{*}{Dataset}& Missing &\multicolumn{2}{c|}{Method}\\
    \cline{3-4}
    &rate& GCN & +\nodenormone \\
    \hline
    \multirow{2}{*}{Cora} & 100 & 0.0235  & 0.0122 \\
    \cline{2-4}
     & 80 &0.0398 & 0.0183 \\
    \hline
    \multirow{2}{*}{Citeseer} & 100 & 0.0226 & 0.0234 \\
    \cline{2-4}
     & 80 & 0.0499 & 0.0204 \\
    \hline
    \multirow{2}{*}{Pubmed} & 100 & 0.0678 & 0.0904 \\    \cline{2-4}
     & 80 & 0.0308 & 0.0225 \\
    \hline
    \end{tabular}
\end{table}
% tab 3 std
\begin{table}[h]
    \centering
    \caption{Standard deviation of results in Tab.~3.}
    \label{tab:low-label-rate-supp}
    \begin{tabular}{|c|c|c|c|}
    \hline
         \multirow{2}{*}{Dataset}& \#Labels &\multicolumn{2}{c|}{Method}\\
    \cline{3-4}
    &per class& GCN & +\nodenormone \\
    \hline
    \multirow{2}{*}{Cora} & 5 & 0.0221 & 0.0178 \\
    \cline{2-4}
     & 2 & 0.0982 & 0.0301\ \\
    \hline
    \multirow{2}{*}{Citeseer} & 5 & 0.0354 & 0.0104 \\
    \cline{2-4}
     & 2 & 0.0695 & 0.0702 \\
    \hline
    \multirow{2}{*}{Pubmed} & 5 & 0.0282 &  0.0191 \\
    \cline{2-4}
     & 2 & 0.0675 & 0.0350  \\
    \hline
    \end{tabular}
\end{table}
% \newpage
% tab 4 std
\begin{table}[h]
    \centering
    \caption{Standard deviation of results in Tab.~4.}
    \begin{tabular}{|c|c|c|}
    \hline
         &GCN&+\nodenormone \\
         \hline
         USelect-12 & 0.0147 & 0.0099 \\
         \hline 
         USelect-16 & 0.0094 & 0.0063 \\
    \hline
    \end{tabular}
\end{table}
% tab 6 std
\begin{table}[h]
    \caption{Standard deviation of results in Tab.~6.}
    \centering
\begin{tabular}{|c|c|}
\hline
Method & AUC-ROC \\
\hline
GEN & 0.0086  \\
\hline
GEN+LayerNorm & 0.0029  \\
\hline
GEN+\nodenormone & 0.0035\\
\hline
\end{tabular}
\end{table}
% tab 7 std
\begin{table}[h]
\caption{Standard deviation of results in Tab.~7.} 
% \label{tab:improving-gcnii}
\centering
 \begin{tabular}{|c|c|c|c|}
\hline
\multirow{2}{*}{Method} & \multicolumn{3}{c|}{Dataset} \\
\cline{2-4}
& Cornell & Texas & Wisconsin\\
\hline
%Dataset & Cornell & Texas & Wisconsin\\
%\hline
GCNII & 0.0514 & 0.0793 & 0.0526 \\
\hline
GCNII+\nodenormone &  0.0692& 0.0637 &  0.0542\\
\hline
\end{tabular}
\end{table}
\newpage

\begin{figure}[h]
    \centering
    \includegraphics[width=\linewidth]{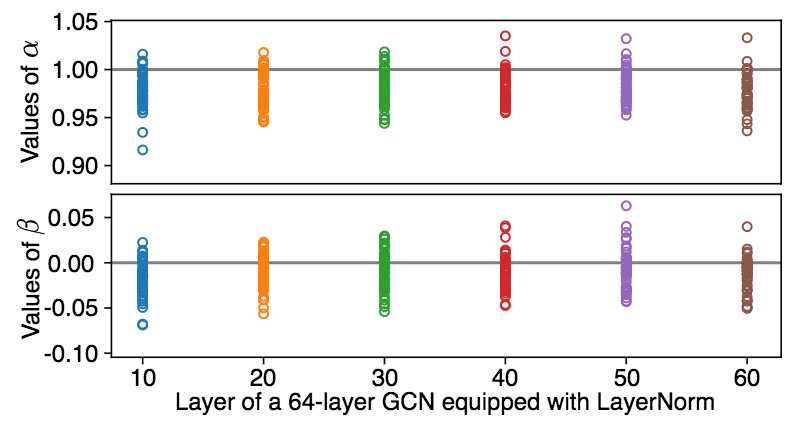}
    \caption{Visualization of learned parameters in LayerNorm. Each single circlet represents the value of a feature dimension, \ie, an entry of $\mathbf{\alpha}$ or $\mathbf{\beta}$.}
    \label{fig:my_label}
\end{figure}

\clearpage
\begin{figure*}[h]
\centering
    \includegraphics[width=\linewidth]{Figures/supp/overfitting_citeseer.png}
    \captionof{figure}{\nodenormone reduces overfitting. Results are on Citeseer.}
\end{figure*}
\begin{figure*}[h]
\centering
    \includegraphics[width=\linewidth]{Figures/supp/overfitting_pubmed.png}
    \captionof{figure}{\nodenormone reduces overfitting. Results are on Pubmed.}
\end{figure*}

\clearpage
\onecolumn
% GCN node1
\begin{table*}[h]
\caption{Hyperparameters of Fig.~3 (GCNs with \nodenormone)}
% \label{}
\centering
\resizebox{0.75\linewidth}{!}{
\begin{tabular}{lcccccc}
     \toprule
     Dataset & \# layers  & dropout rate & $\ell_1$ weight & weight decay factor & learning rate & \# epochs\\
     \midrule
     \multirow{6}{*}{Cora}&2	&0.8	&0.0005	&0.0005 &0.005&400\\
&4	&0.6	&0.01	&0.0005 &0.005&400\\
&8	&0.7	&0.005	&0.001 &0.005&400\\
&16	&0.8	&0.001	&0.001 &0.005&400\\
&32	&0.7	&0.001	&0.0005 &0.005&400\\
&64	&0.5	&0.0005	&0.001 &0.005&400\\
    \midrule
    \multirow{6}{*}{Citeseer}&2	&0.6	&0.01	&0.0005 &0.005&400\\
&4	&0.6	&0.01	&0.001 &0.005&400\\
&8	&0.5	&0.005	&0.001 &0.005&400\\
&16	&0.6	&0.001	&0.001 &0.005&400\\
&32	&0.6	&0.005	&0.001 &0.005&400\\
&64	&0.6	&0.01	&0.001 &0.005&400\\
    \midrule
    \multirow{6}{*}{Pubmed}&2	&0.7	&0.005	&0.0005 &0.005&400\\
&4	&0.6	&0.005	&0.0005 &0.005&400\\
&8	&0.8	&0.005	&0.001 &0.005&400\\
&16	&0.6	&0.01	&0.001 &0.005&400\\
&32	&0.5	&0.005	&0.0005 &0.005&400\\
&64	&0.7	&0.005	&0.0005 &0.005&400\\
    \midrule
    \multirow{6}{*}{Coauthor-CS}&2		&0	    &0.0005	&0.001          &0.005&400	\\
&4		&0.6	&0.0001	&0.001          &0.005&400	\\
&8		&0.5	&0.0001	&0.0005          &0.005&400	\\
&16		&0.5	&0	    &0.001          &0.005&400	\\
&32		&0.6	&0	    &0.0005          &0.005&400	\\
&64		&0.5	&0	    &0.001            &0.005&400	\\
    \midrule
    \multirow{6}{*}{Wiki-CS}&2&0.3&	0	    &0.0005   &0.005  &400 \\  
&4&0.3&	0.0001	&0.0005  &0.005  &400 \\ 
&8&0.5&	0	    &0.001    &0.005  &400 \\ 
&16&0.3&	0.0001	&0.001    &0.005  &400 \\ 
&32&0.3&	0	    &0.001    &0.005  &400 \\ 
&64&0.3&	0	    &0.001  	 &0.005  &400 \\ 
    \midrule
    \multirow{6}{*}{Amazon-photo}&2		&0.5	&0.0005	&0.0005		&0.005 &400 \\				
&4		&0.8	&0.001	&0.0005		&0.005 &400 \\				
&8		&0.8	&0.0005	&0.001	    &0.005 &400 \\				
&16		&0.7	&0.001	&0.001		&0.005 &400 \\				
&32		&0.6	&0.001	&0.0005		&0.005 &400 \\				
&64		&0.5	&0.0001	&0.001		&0.005 &400 \\	
    \midrule
\bottomrule                         
\end{tabular}
}
\end{table*}
% GCN node2
\begin{table*}[htbp]
\caption{Hyperparameters of Fig.~3 (GCNs with \nodenormtwo)}
% \label{}
\centering
\resizebox{0.7\linewidth}{!}{
\begin{tabular}{lcccccc}
     \toprule
     Dataset & \# layers  & dropout rate & $\ell_1$ weight & weight decay factor & learning rate & \# epochs\\
     \midrule
     \multirow{6}{*}{Cora}&2	&0.8	&0.0001	&0.0005 &0.005&400\\
&4	&0.8	&0.001	&0.001 &0.005&400\\
&8	&0.8	&0.0005	&0.001 &0.005&400\\
&16	&0.8	&0.001	&0.001 &0.005&400\\
&32	&0.6	&0.005	&0.0005 &0.005&400\\
&64	&0.5	&0.01	&0.0005 &0.005&400\\
    \midrule
    \multirow{6}{*}{Citeseer}&2	&0.8	&0.0005	&0.001 &0.005&400\\
&4	&0.6	&0.005	&0.0005 &0.005&400\\
&8	&0.8	&0.001	&0.0005 &0.005&400\\
&16	&0.8	&0.001	&0.0005 &0.005&400\\
&32	&0.8	&0.001	&0.001 &0.005&400\\
&64	&0.5	&0.005	&0.0005 &0.005&400\\
    \midrule
    \multirow{6}{*}{Pubmed}&2	&0.6	&0.001	&0.0005 &0.005&400\\
&4	&0.8	&0.0005	&0.0005 &0.005&400\\
&8	&0.6	&0.001	&0.0005 &0.005&400\\
&16	&0.7	&0.005	&0.001 &0.005&400\\
&32	&0.5	&0.01	&0.001 &0.005&400\\
&64	&0.6	&0.005	&0.0005 &0.005&400\\
    \midrule
    \multirow{6}{*}{Coauthor-CS}&2		&0.6	&0	    &0.001          &0.005&400	\\
&4		&0.5	&0.0001	&0.0005          &0.005&400	\\
&8		&0.7	&0.0001	&0.0005          &0.005&400	\\
&16		&0.7	&0.0001	&0.001          &0.005&400	\\
&32		&0.6	&0	    &0.0005          &0.005&400	\\
&64		&0.7	&0	    &0.001          &0.005&400	\\
    \midrule
    \multirow{6}{*}{Wiki-CS}&2&0.6&	0	    &0.0005   &0.005  &400 \\  
&4&0.6&	0.0001	&0.0005   &0.005  &400 \\  
&8&0.6&	0	    &0.001    &0.005  &400 \\ 
&16&0.5&	0.0001	&0.001    &0.005  &400 \\ 
&32&0.3&	0.0001	&0.0005   &0.005  &400 \\  
&64&0.3&	0.005	&0.0005   &0.005  &400 \\
    \midrule
    \multirow{6}{*}{Amazon-photo}&2		&0.7	&0.0005	&0.001		&0.005 &400 \\					
&4		&0.6	&0.001	&0.0005		&0.005 &400 \\					
&8		&0.5	&0.0005	&0.0005		&0.005 &400 \\					
&16		&0.6	&0.001	&0.0005	    &0.005 &400 \\					
&32		&0.6	&0.005	&0.001		&0.005 &400 \\					
&64		&0	&0.01	&0.001		&0.005 &400 \\	
    \midrule
\bottomrule                         
\end{tabular}
}
\end{table*}
% GCN node3
\begin{table*}[htbp]
\caption{Hyperparameters of Fig.~3 (GCNs with \nodenormthree)}
% \label{}
\centering
\resizebox{0.7\linewidth}{!}{
\begin{tabular}{lcccccc}
     \toprule
     Dataset & \# layers  & dropout rate & $\ell_1$ weight & weight decay factor & learning rate & \# epochs\\
     \midrule
     \multirow{6}{*}{Cora}&2		&0.8	&0.0001	&0.0005   &0.005&400\\
&4		&0.8	&0.001	&0.0005   &0.005&400\\
&8		&0.8	&0.001	&0.0005   &0.005&400\\
&16		&0.7	&0.001	&0.001   &0.005&400\\
&32		&0	   &0.005	&0.0005   &0.005&400\\
&64		&0	   &0.005	&0.0005   &0.005&400\\

    \midrule
    \multirow{6}{*}{Citeseer}&2		&0.8	&0.0001	&0.0005   &0.005&400\\
&4		&0.8	&0.001	&0.0005   &0.005&400\\
&8		&0.8	&0.001	&0.001   &0.005&400\\
&16		&0.8	&0.001	&0.0005   &0.005&400\\
&32		&0.5	&0.001	&0.0005   &0.005&400\\
&64		&0.5	&0.005	&0.001   &0.005&400\\
    \midrule
    \multirow{6}{*}{Pubmed}&2		&0.6	&0.0005	&0.0005   &0.005&400\\
&4		&0.7	&0.001	&0.0005   &0.005&400\\
&8		&0.7	&0.0005	&0.0005   &0.005&400\\
&16		&0.6	&0.005	&0.0005   &0.005&400\\
&32		&0.5	&0.001	&0.0005   &0.005&400\\
&64		&0.6	&0.005	&0.001   &0.005&400\\
    \midrule
    \multirow{6}{*}{Coauthor-CS}&2		&0.5	&0	    &0.001          &0.005&400	\\
&4		&0.5	&0.001	&0.0005          &0.005&400	\\
&8		&0.5	&0	    &0.0005          &0.005&400	\\
&16		&0.8	&0	    &0.001          &0.005&400	\\
&32		&0.5	&0.0005	&0.0005          &0.005&400	\\
&64		&0.5	&0.0005	&0.001          &0.005&400	\\
    \midrule
    \multirow{6}{*}{Wiki-CS}&2&0.5&	0 	&0.001    &0.005  &400 \\ 
&4&0.6&	0	    &0.001    &0.005  &400 \\
&8&0.5&	0	    &0.0005   &0.005  &400 \\     
&16&0.3&	0.0005	&0.001    &0.005  &400 \\     
&32&0.7&	0.0001	&0.001    &0.001  &1500\\  
&64&0.6&	0	    &0.0005   &0.001  &1500\\  
    \midrule
    \multirow{6}{*}{Amazon-photo}&2		&0.5	&0.0005	&0.0005		&0.005 &400 \\					
&4		&0.5	&0.001	&0.001		&0.005 &400 \\					
&8		&0.6	&0.0005	&0.001		&0.005 &400 \\					
&16		&0.5	&0.005	&0.001		&0.005 &400 \\					
&32		&0	&0.01	&0.001		&0.005 &400 \\								
&64		&0	&0.0005	&0.0005		&0.005 &400 \\
    \midrule
\bottomrule                         
\end{tabular}
}
\end{table*}
% GCN layer
\begin{table*}[htbp]
\caption{Hyperparameters of Fig.~3 (GCNs with LayerNorm)}
% \label{}
\centering
\resizebox{0.7\linewidth}{!}{
\begin{tabular}{lcccccc}
     \toprule
     Dataset & \# layers  & dropout rate & $\ell_1$ weight & weight decay factor & learning rate & \# epochs\\
     \midrule
     \multirow{6}{*}{Cora}&2	&0.7	&0.001	&0.0005 &0.005&400\\
&4	&0.8	&0.001	&0.0005 &0.005&400\\
&8	&0.8	&0.001	&0.001 &0.005&400\\
&16	&0.8	&0.001	&0.001 &0.005&400\\
&32	&0.8	&0.005	&0.001 &0.005&400\\
&64	&0.5	&0.001	&0.001 &0.005&400\\
    \midrule
    \multirow{6}{*}{Citeseer}&2	&0.6	&0.01	&0.001 &0.005&400\\
&4	&0.6	&0.005	&0.001 &0.005&400\\
&8	&0.5	&0.005	&0.0005 &0.005&400\\
&16	&0.5	&0.005	&0.0005 &0.005&400\\
&32	&0.8	&0.0005	&0.001 &0.005&400\\
&64	&0.7	&0.005	&0.001 &0.005&400\\
    \midrule
    \multirow{6}{*}{Pubmed}&2	&0.6	&0.01	&0.0005 &0.005&400\\
&4	&0.8	&0.005	&0.001 &0.005&400\\
&8	&0.7	&0.01	&0.001 &0.005&400\\
&16	&0.8	&0.005	&0.001 &0.005&400\\
&32	&0.7	&0.005	&0.001 &0.005&400\\
&64	&0.7	&0.01	&0.001 &0.005&400\\
    \midrule
    \multirow{6}{*}{Coauthor-CS}&2		&0	    &0.0005	&0.001          &0.005&400	\\
&4		&0.5	&0.0001	&0.001          &0.005&400	\\
&8		&0.6	&0.0001	&0.0005          &0.005&400	\\
&16		&0.6	&0.0001	&0.0005          &0.005&400	\\
&32		&0.6	&0.0001	&0.0005          &0.005&400	\\
&64		&0.5	&0  	&0.001          &0.005&400	\\
    \midrule
    \multirow{6}{*}{Wiki-CS}&2&0.5&	0	    &0.0005  &0.005  &400 \\ 
&4&0.7&	0   	&0.0005  &0.005  &400 \\  
&8&0.7&	0   	&0.0005  &0.005  &400 \\   
&16&0.6&	0	    &0.001   &0.005  &400 \\  
&32&0.7&	0	    &0.0005  &0.005  &400 \\  
&64&0.6&	0.0001&	0.0005	 &0.005  &400 \\ 	
    \midrule
    \multirow{6}{*}{Amazon-photo}&2		&0.7	&0.001	&0.001		&0.005 &400 \\				
&4		&0.5	&0.005	&0.0005		&0.005 &400 \\				
&8		&0.7	&0.001	&0.0005	    &0.005 &400 \\				
&16		&0.5	&0.001	&0.0005		&0.005 &400 \\				
&32		&0.6	&0.001	&0.0005		&0.005 &400 \\				
&64		&0.6	&0.0005	&0.001		&0.005 &400 \\
    \midrule
\bottomrule                         
\end{tabular}
}
\end{table*}
% missing features
\begin{table*}[htbp]
\caption{Hyperparameters of Tab.~2 (GCN with \nodenormone on citation graphs with missing features).}
% \label{}
\centering
\resizebox{0.7\linewidth}{!}{
\begin{tabular}{lccccccc}
     \toprule
     Dataset & Missing rate(\%)  & dropout rate & $\ell_1$ weight & weight decay factor & learning rate &\# epochs & Best layer\\
     \midrule
     \multirow{2}{*}{Cora}& 100&0.6 & 0.01& 0.001  &0.005 &1500& 64\\ 
                         &80&0.8 &0.001 &0.0005 &0.005 & 1500 & 64\\
    \midrule
    \multirow{2}{*}{Citeseer}& 100& 0.5& 0.005& 0.0005& 0.005 &1500 &32  \\ 
                         &80&0.6 &0.0001 & 0.001 & 0.005 & 1500 & 32\\
    \midrule
    \multirow{2}{*}{Pubmed}& 100&0.5 &0 &0.0005 &0.005 &1500 &16 \\ 
                         &80&0.8 &0.001 &0.001  & 0.005& 1500&8 \\
\bottomrule                         
\end{tabular}
}
\end{table*}
% low label rate
\begin{table*}[htbp]
\caption{Hyperparameters of Tab.~3 (GCN with \nodenormone on citation graphs with low label rate).}
% \label{}
\centering
\resizebox{0.7\linewidth}{!}{
\begin{tabular}{lccccccc}
     \toprule
     Dataset & \# labels per class  & dropout rate & $\ell_1$ weight & weight decay factor & learning rate &\# epochs & Best layer\\
     \midrule
     \multirow{2}{*}{Cora}& 5& 0.5 & 0.005 & 0.0005 & 0.005  &400 & 8\\ 
                         &2&0.6 & 0.005 & 0.001 &0.005 &400 & 16 \\
    \midrule
    \multirow{2}{*}{Citeseer}& 5& 0.5 &0.001 &0.001 &0.005  &400 &32  \\ 
                         &2&0.7 & 0.01 & 0.001 &0.005 &400 & 16 \\
    \midrule
    \multirow{2}{*}{Pubmed}& 5&0.5 & 0.005&0.001 &0.005 &400 &64 \\ 
                         &2&0.5 & 0.005&0.001 &0.005 &400 &64 \\ 
\bottomrule                         
\end{tabular}
}
\end{table*}
% us election
\begin{table*}[htbp]
\caption{Hyperparameters of Tab.~4 (GCN with \nodenormone on USelect-12 and USelect-16).}
% \label{}
\centering
\resizebox{0.6\linewidth}{!}{
\begin{tabular}{lccccccc}
     \toprule
     Dataset  & dropout rate & $\ell_1$ weight & weight decay factor & learning rate &\# epochs & Best layer\\
     \midrule
     USelect-12&  0& 0&0.0005 &0.01  &1500 & 32\\ 
                      
    \midrule
    USelect-16& 0.6 &0.0005 &0.001 &0.01  &1500 &32  \\ 
                        
\bottomrule                         
\end{tabular}
}
\end{table*}
% compare with sota
\begin{table*}[htbp]
\caption{Hyperparameters of Tab. 5.}
% \label{tab:hypers-tab2}
\centering
\resizebox{0.7\linewidth}{!}{
\begin{tabular}{lcccccc}
     \toprule
     Dataset & \# layers  & dropout rate & $\ell_1$ weight & weight decay factor & learning rate & \# epochs\\
     \midrule
     \multirow{6}{*}{Cora}&2	&0.7	&0.01	&0.0005 &0.005&400\\
&4	&0.7	&0.0005	&0.0003 &0.005&400\\
&8	&0.7	&0.0008	&0.0008 &0.005&400\\
&16	&0	&0.003	&0.001 &0.005&400\\
&32	&0.4	&0.0008	&0.0003 &0.005&400\\
&64	&0.7	&0.008	&0.0005 &0.005&400\\
    \midrule
    \multirow{6}{*}{Citeseer}&2	&0.8	&0.001	&0.001 &0.005&400\\
&4	&0.5	&0.003	&0.0005 &0.005&400\\
&8	&0.9	&0.0005	&0.0001 &0.005&400\\
&16	&0.8	&0.001	&0.001 &0.005&400\\
&32	&0.4	&0.001	&0.0005 &0.005&400\\
&64	&0.6	&0.005	&0.0003 &0.005&400\\
    \midrule
    \multirow{6}{*}{Pubmed}&2	&0.4	&0.005	&0.0001 &0.005&400\\
&4	&0.8	&0.01	&0.001 &0.005&400\\
&8	&0.9	&0.005	&0.0005 &0.005&400\\
&16	&0.7	&0.01	&0.0001 &0.005&400\\
&32	&0	&0.01	&0.0003 &0.005&400\\
&64	&0.9	&0.003	&0.0003 &0.005&400\\

\bottomrule                         
\end{tabular}
}
\end{table*}

% in-conv implementation
% \begin{table*}[htbp]
% \caption{Hyperparameters of training 64-layer GCNs with \nodenormonein or LayerNorm-In.}
% % \label{}
% \centering
% \resizebox{0.7\linewidth}{!}{
% \begin{tabular}{lcccccc}
%      \toprule
%      Dataset & Method  & dropout rate & $\ell_1$ weight & weight decay factor & learning rate & \# epochs\\
%      \midrule
%      \multirow{2}{*}{Cora}& \nodenormonein& & & & &  \\ 
%                          &LayerNorm-In& & &  & &  \\
%     \midrule
%     \multirow{2}{*}{Citeseer}& \nodenormonein& & & & &  \\ 
%                          &LayerNorm-In& & &  & &  \\
%     \midrule
%     \multirow{2}{*}{Pubmed}& \nodenormonein& & & & &  \\ 
%                          &LayerNorm-In& & &  & &  \\
% \bottomrule                         
% \end{tabular}
% }
% \end{table*}
\clearpage
